# Supplementary material for: Unifying the description of hydrocarbons and hydrogenated carbon materials with a chemically reactive machine learning interatomic potential
Source: arXiv:2409.08194 source file (2024-09-12)
Supplement: Supplementary file 1 [file Suplementary.tex]

\documentclass{article}
\usepackage[utf8]{inputenc}
\usepackage{amsmath}
\usepackage{graphicx}
\usepackage{caption}
\usepackage{epstopdf}
\usepackage[section]{placeins}
\usepackage{fancyhdr}
\usepackage[left=2.0cm,right=2.0cm,top=2.3cm,bottom=2.2cm]{geometry}
\pagestyle{fancy}

\title{Supporting Information for "Unifying the description of hydrocarbons and hydrogenated carbon materials with a
chemically reactive machine learning interatomic potential"}
\author{Rina Ibragimova, Mikhail S. Kuklin, Tigany Zarrouk, and Miguel A. Caro}
\date{}

\begin{document}

\maketitle

\begin{table}[h]
\centering
\begin{tabular}{|c c|} 
 \hline
 Structure type & Regularization $\sigma$ energy (eV/atom) \\ 
 \hline
 QM9 & 0.0001 \\ 
 \hline
 QM9 distorted & 0.001 \\ 
 \hline
 Bulk C & 0.0001 \\
 \hline
 Amorphous C & 0.001 \\ 
 \hline
 Amorphous surface C & 0.001 \\ 
 \hline
 Melt-quench & 0.005\\
 \hline
 High pressure & 0.001\\
 \hline
 Interacting molecules & 0.0001\\
 \hline
 Soup (first iteration) & 0.025\\
 \hline
 Soup (last iteration) & 0.001\\
 \hline
  Other structures (default) & 0.001\\
 \hline
\end{tabular}
\caption{Summary of regularization values for different structures in the training dataset.}
\label{table:reg_summary}
\end{table}

\begin{figure*}[ht!]
\centering
\includegraphics[width=0.9\textwidth]{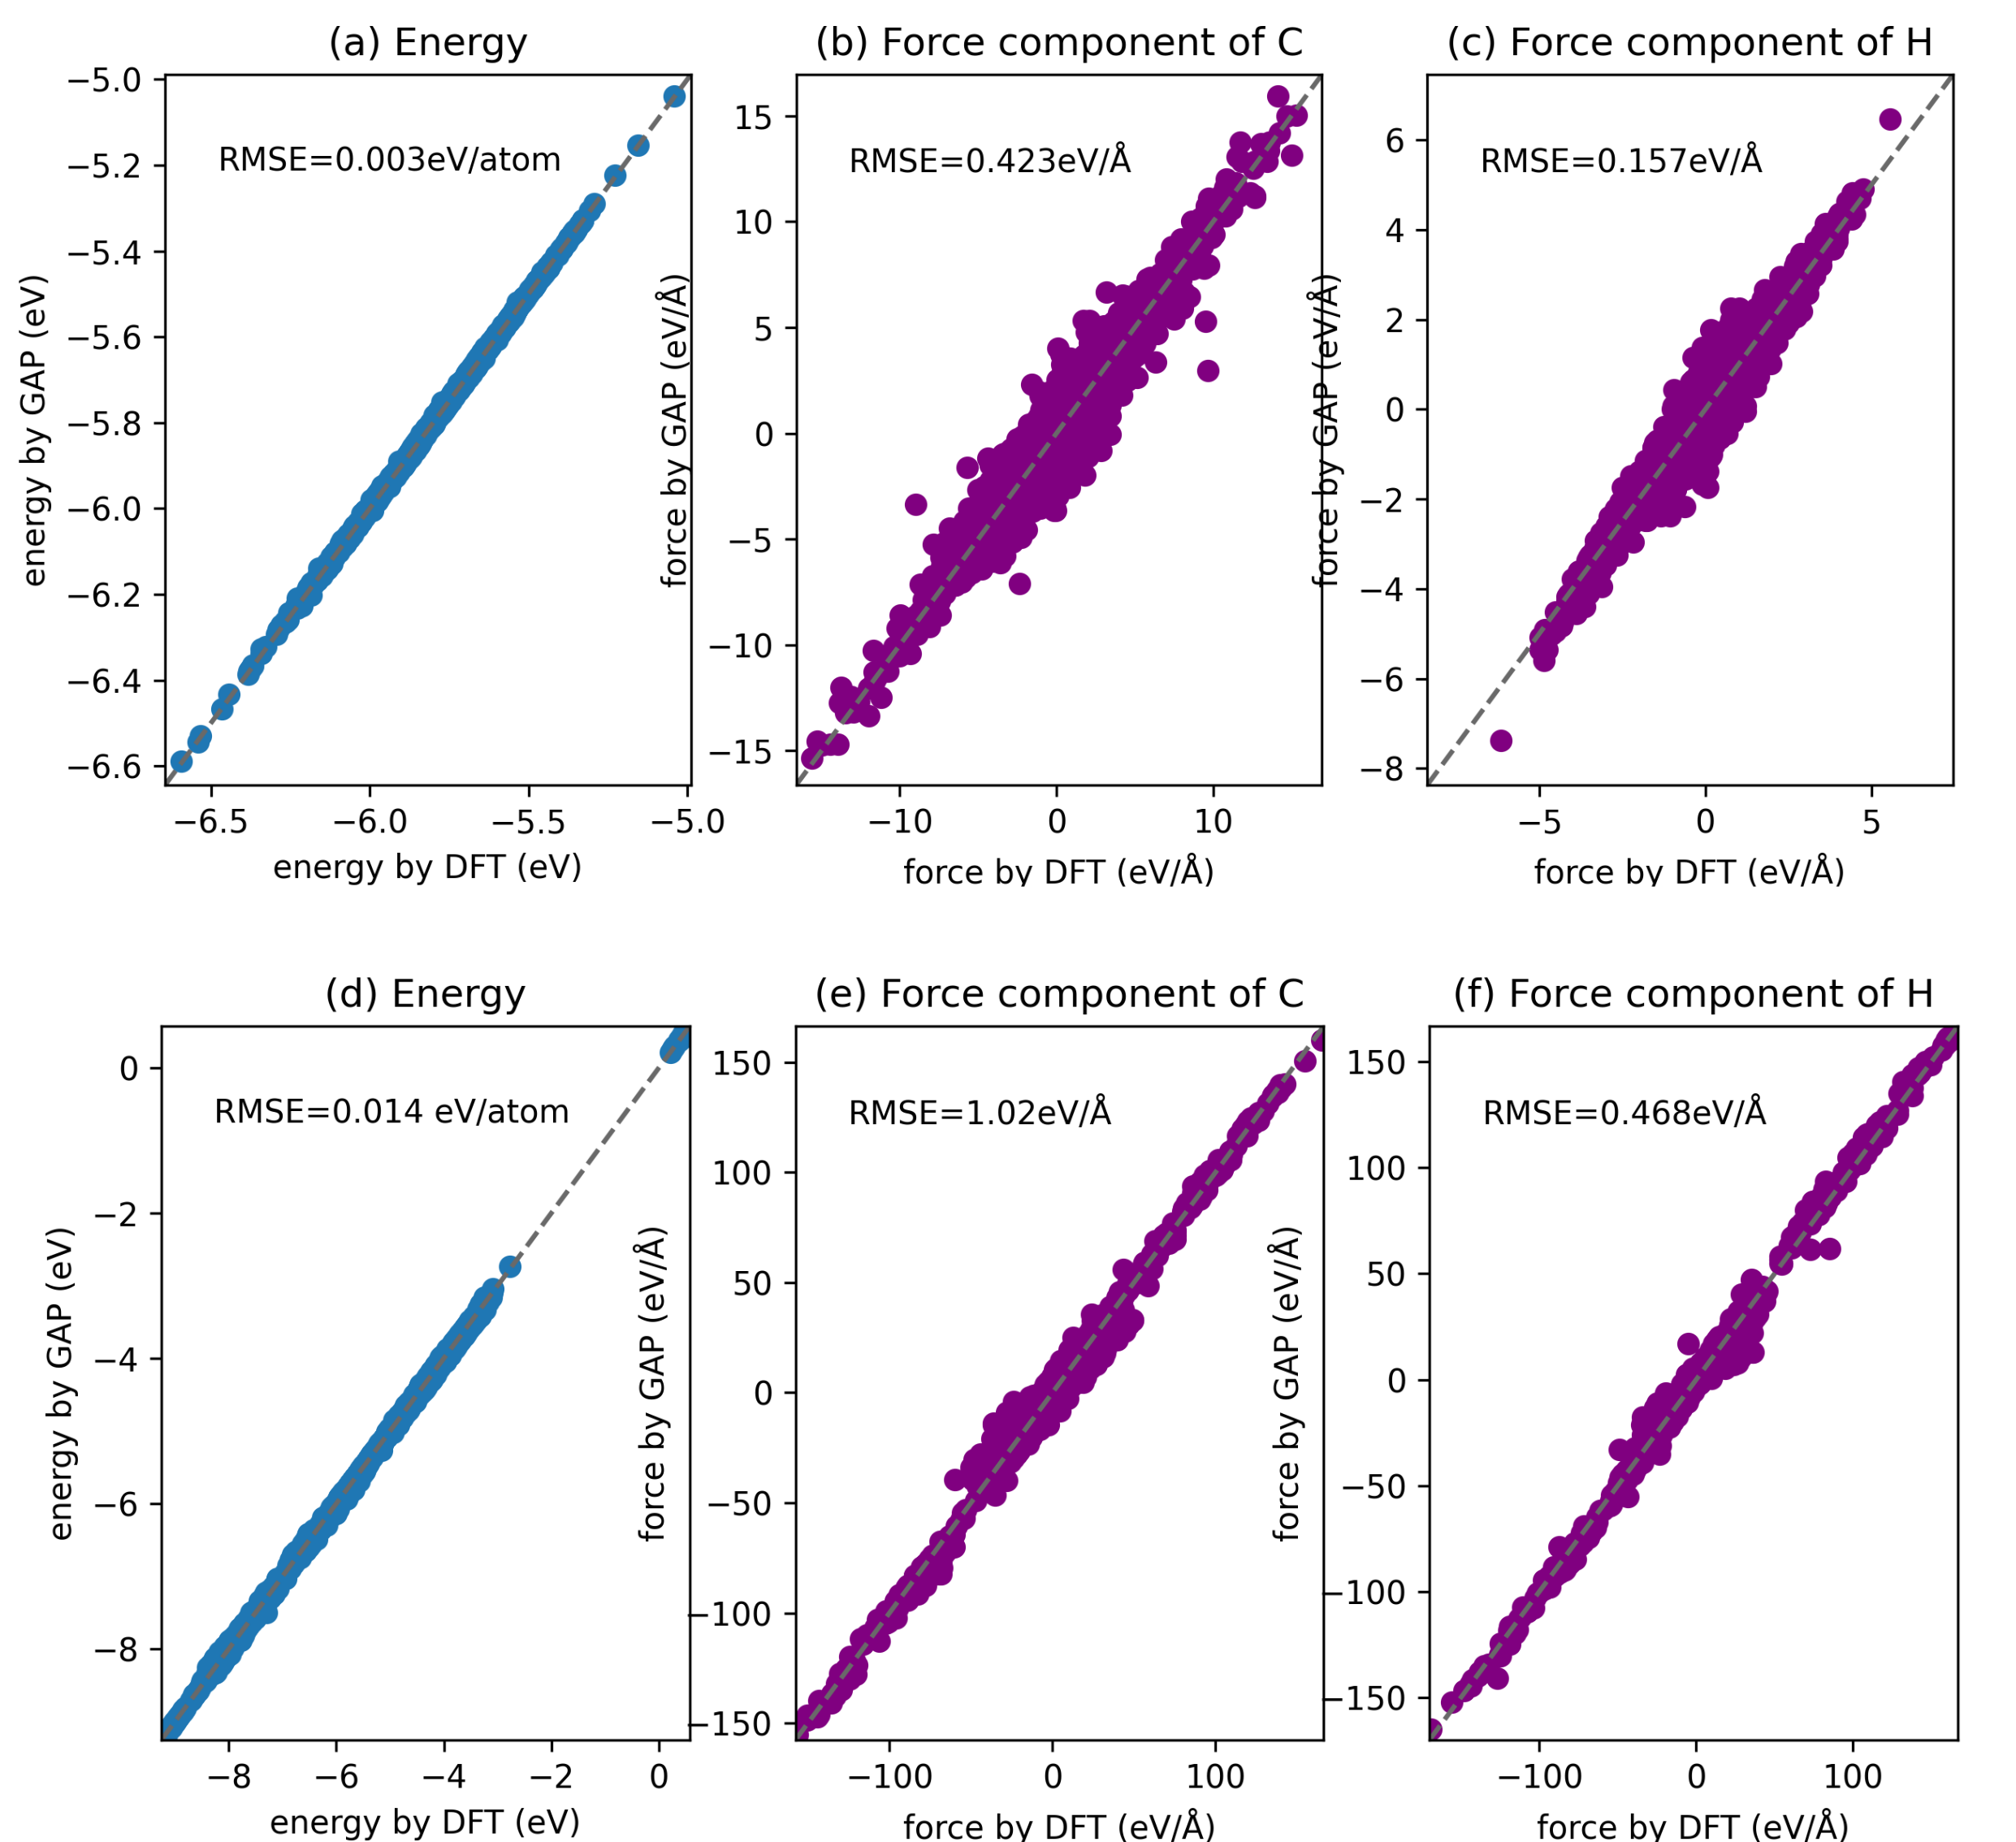}
\caption{\label{fig:scatter} Scatterplots comparing DFT calculations with the prediction from GAP. (a) GAP energy \textit{vs.} DFT energy, (b), and (c) force components of C, and H for QM9 database. And the data for a test set of structures, which were not included in the
ﬁt (d) GAP energy \textit{vs.} DFT energy, (e) force components of C, and (f) H for 20\% of test split.}

\end{figure*}

\end{document}
